# Supplementary material for: A Review of Indoor Millimeter Wave Device-based Localization and Device-free Sensing Technologies and Applications
Source: arXiv:2112.05593 source file (2022-05-25)
Supplement: Supplementary file 1 [file appendices_file.tex]

\appendices

Appendix one text goes here.

% you can choose not to have a title for an appendix
% if you want by leaving the argument blank
\section{}
Appendix two text goes here.
